# Supplementary material for: Analysis of Indexing Structures for Immutable Data
Source: arXiv:2003.02090 source file (2020-03-10)
Supplement: Supplementary file 1 [file appendix.tex]

{\em chunk-based deduplication} can be conducted at different granularity.
One simple approach is to find duplicates at whole file level, e.g. git, SIS~\cite{bolosky:2000}, where identical files are kept as a single copy.
While the approach does not require additional data partitioning logic, the deduplication gain is limited as one small modification in the file will cause the system to create a new file.
Another approach is to partition the data to fixed-size chunks e.g. Venti~\cite{Quinlan:2002}, \cite{Hong:2004}.
Fixed-size chunking provides better deduplication gain, while the index space increases with more fine-grained chunk size, causing more processing overhead.
Moreover, update in one chunk may cause all following chunks to be re-partitioned, i.e. boundary-shifting problem~\cite{eshghi:2005}.
Regarding to this, content-defined chunking is introduced. 
\cite{muthitacharoen:2001} calculate Rabin Fingerprint within a sliding window and use it to determines the data partitioning boundary. Two Threshold Two Divisor (TTTD)~\cite{eshghi:2005} was proposed to further reduce boundary shifting problems when basic sliding window approach cannot find boundary. TTTD-S~\cite{Moh:2010} improves TTTD by reducing the variance in the chunk size created by TTTD and mitigating the processing overhead.
\cite{Kruus:2010} and \cite{Lu:2010} reduce the number of chunks created by modeling the modification frequency, combining the unchanged chunks and splitting the modified chunks.
In addition, collaborative analytic engines
deduplicate at sub-table level.
Decibel~\cite{maddox:2016} studies differences between
row/column-based schemes,
while OrpheusDB~\cite{xu:2017} applies an advanced partitioning
strategy to tune tradeoff between checkout time and space consumption.
